# Supplementary material for: Systems and Methods for the Spectral Calibration of Swept Source Optical Coherence Tomography Systems
Source: arXiv:2002.08755 source file (2019-12-02)
Supplement: Supplementary file 1 [file appendices.tex]

%%%%%%%%%%%%%%%%%%%%%%%%%%%%%%%%%%%%%%%%%%%%%%%%%%%
%
%  New template code for TAMU Theses and Dissertations starting Fall 2016.  
%
%
%  Author: Sean Zachary Roberson
%  Version 3.17.09
%  Last Updated: 9/21/2017
%
%%%%%%%%%%%%%%%%%%%%%%%%%%%%%%%%%%%%%%%%%%%%%%%%%%%

\begin{appendices}
\titleformat{\chapter}{\centering\normalsize}{APPENDIX \thechapter}{0em}{\vskip .5\baselineskip\centering}

%%%%%%%%%%%%%%%%%%%%%%%%%%%%%%%%%%%%%%%%%%%%%%%%%%%
%
%  New template code for TAMU Theses and Dissertations starting Fall 2016.
%
%
%  Author: Sean Zachary Roberson 
%	 Version 3.16.09
%  Last updated 9/12/2016
%
%%%%%%%%%%%%%%%%%%%%%%%%%%%%%%%%%%%%%%%%%%%%%%%%%%%

%%%%%%%%%%%%%%%%%%%%%%%%%%%%%%%%%%%%%%%%%%%%%%%%%%%%%%%%%%%%%%%%%%%%%%
%%                           APPENDIX A 
%%%%%%%%%%%%%%%%%%%%%%%%%%%%%%%%%%%%%%%%%%%%%%%%%%%%%%%%%%%%%%%%%%%%%

\phantomsection

\chapter{\uppercase{First Appendix}}

Text for the Appendix follows.

\begin{figure}[h]
\centering
\includegraphics[scale=.50]{figures/Penguins.jpg}
\caption{TAMU figure}
\label{fig:tamu-fig5}
\end{figure}

%%%%%%%%%%%%%%%%%%%%%%%%%%%%%%%%%%%%%%%%%%%%%%%%%%%
%
%  New template code for TAMU Theses and Dissertations starting Fall 2016.
%
%
%  Author: Sean Zachary Roberson 
%	 Version 3.16.09 
%  Last updated 9/12/2016
%
%%%%%%%%%%%%%%%%%%%%%%%%%%%%%%%%%%%%%%%%%%%%%%%%%%%

%%%%%%%%%%%%%%%%%%%%%%%%%%%%%%%%%%%%%%%%%%%%%%%%%%%%%%%%%%%%%%%%%%%%%%
%%                           APPENDIX B
%%%%%%%%%%%%%%%%%%%%%%%%%%%%%%%%%%%%%%%%%%%%%%%%%%%%%%%%%%%%%%%%%%%%%

\chapter{\uppercase {A Second Appendix Whose Title Is Much Longer Than The First}}

Text for the Appendix follows.

\begin{figure}[h]
\centering
\includegraphics[scale=.50]{figures/Penguins.jpg}
\caption{Another TAMU figure.}
\label{fig:tamu-fig6}
\end{figure}

\section{Appendix Section}

\section{Second Appendix Section}

\pagebreak{}

\end{appendices}
